# Supplementary material for: Accurate exchange-correlation energies for the warm dense electron gas
Source: arXiv:1602.05104 ancillary file (2016-09-10)
Supplement: Supplementary file 1 [file supp.pdf]

# Supplementary Material: Accurate exchange-correlation energies for the warm dense electron gas

## I. APPROXIMATIONS

### A. Initiator Approximation

The critical populations necessary to overcome the sign problem at low temperatures are too large for most systems of interest and approximations are therefore required. We use an analogue of the initiator approximation developed for the FCIMQC method ($i$-FCIQMC) [1], which has been used in a variety of successful chemical [2–4], model [5, 6] and solid-state FCIQMC simulations [7] and has been applied to UEG systems of up to 54 unpolarized electrons at zero temperature [5, 6]. Here we find it equally useful at finite temperature. While spawning to already-occupied determinants is unaffected, the initiator approximation only allows spawning events to unoccupied determinants that originate from a set of 'initiator determinants' with walker populations above a certain threshold, $n_{\text{add}}$, or that result from multiple sign-coherent spawning events from non-initiator determinants. The effects of the initiator approximation may be reduced by increasing the total walker population, $N_w$, with the original DMQMC algorithm recovered as $N_w \to \infty$.

In DMQMC, due to the sparse sampling of the initial condition, a direct application of the initiator approximation can lead to incorrect averages at higher temperatures. This happens when the $i$-DMQMC algorithm has too little imaginary time to determine the initiator space dynamically. While the results should still be valid in the $N_w \to \infty$ limit, the rate of convergence to this limit can be slow. To ameliorate this problem, we permanently set all density matrix elements at excitation levels $n_{\text{ex}} \leq 2$ to be initiators. (A density matrix element at excitation level $n_{\text{ex}}$ is one for which the bra and the ket differ by $n_{\text{ex}}$ particle-hole pairs.) This reduces the effect of the initiator approximation in the early stages of the simulation, before the initiator distribution has been properly determined. At lower temperatures, this modification becomes less important as the initial walker population occupies a relatively small number of low-energy diagonal density matrix elements. The effects of introducing a permanent initiator space can be monitored by ensuring that the results do not change significantly as its size is increased. Unfortunately, we found that the initiator approximation can lead to poor convergence for operators which do not commute with the Hamiltonian and they are thus omitted from Table II.

In Table I we demonstrate the convergence as a function of $N_w$ of the initiator error in the $i$-DMQMC estimate of the internal energy of a 33–electron, spin-polarised system with $r_s = 0.6, 1, 2$ and $\Theta = 0.0625$. Any bias is essentially negligible (estimated at less than 1%) for $N_w > 10^6$ and much smaller than $k_B T$.

Figs. 1 and 2 show the convergence of the $i$-DMQMC internal energy with particle number for different basis sizes. We see that the convergence is in general non-monotonic and care needs to be taken to ensure convergence is achieved. Notwithstanding these issues, we see that the initiator error is very small ($\approx 1$ milli-Hartree per-particle) for $N_w \geq 10^4$ and for the system considered here. We also see that the initiator error is well controlled for comparing to CPIMC (and by RPIMC).

Fig. 3 on the other hand, demonstrates that the initiator approximation is also applicable to higher temperatures, although any obvious trend can often be masked by the naturally larger error bars as the temperature is increased.

| | $r_s$ | | |
|---|---|---|---|
| $N_w$ | 0.6 | 1 | 2 |
| $1 \times 10^4$ | 3.8894(2) | 1.1458(2) | 0.12491(5) |
| $1 \times 10^5$ | 3.8899(1) | 1.1460(2) | 0.12423(9) |
| $1 \times 10^6$ | 3.8893(2) | 1.1455(2) | 0.12223(7) |
| $5 \times 10^6$ | 3.8893(2) | 1.1452(2) | 0.1211(5) |

TABLE I. Convergence of the $i$-DMQMC internal energy per particle with the target walker number, $N_w$, for $\Theta = 0.0625$, $N = 33$ and $M = 1045$ at a variety of $r_s$ values with $n_{\text{add}} = 3$. For $r_s = 2$ we used $n_{\text{ex}} = 0$ and grew the population past $N_w = 10^5$, whilst for $r_s = 0.6, 1$ we used $n_{\text{ex}} = 2$ and kept the population fixed at $N_w$. The initiator error is typically smaller than 1 milli-Hartree per particle at $N_w > 10^6$.

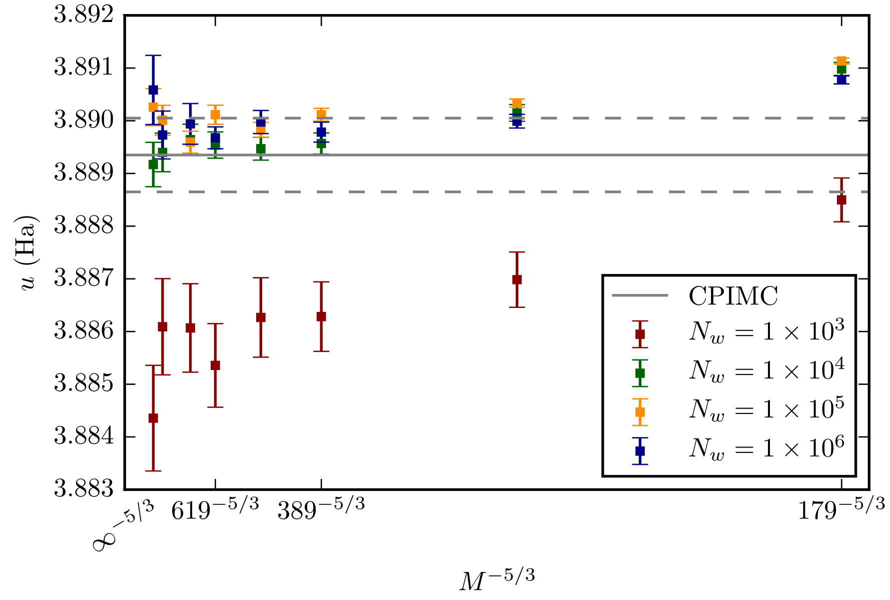


FIG. 1. Convergence of $i$-DMQMC internal energy with basis set size ($M$) while varying the target walker population ($N_w$) for $N = 33$, $r_s = 0.6$, $\Theta = 0.0625$. Here the asymmetric equations of motion were used and we ran with a fixed population. Also plotted is the CPIMC energy (solid line) and 1-$\sigma$ error bars (dashed lines).

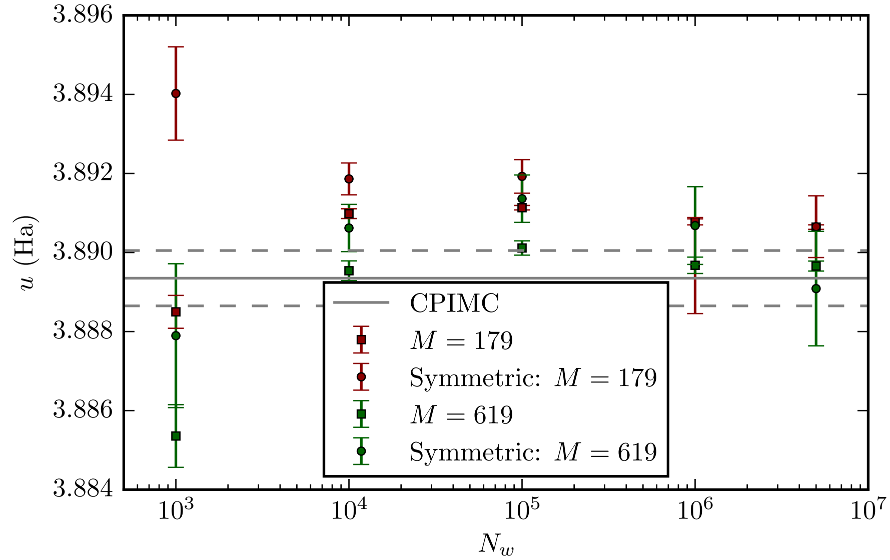


FIG. 2. Convergence of $i$-DMQMC internal energy with target population ($N_w$) for $N = 33$, $r_s = 0.6$, $\Theta = 0.0625$ for two different basis set sizes ($M$). We see that the convergence of initiator error generally differs when using either the symmetric (squares) or asymmetric (circles) equations of motion, however both methods produce identical results in the large $N_w$ limit. The shift was varied throughout. Also plotted is the CPIMC energy (solid line) and 1-$\sigma$ error bars (dashed lines) from Ref [8].

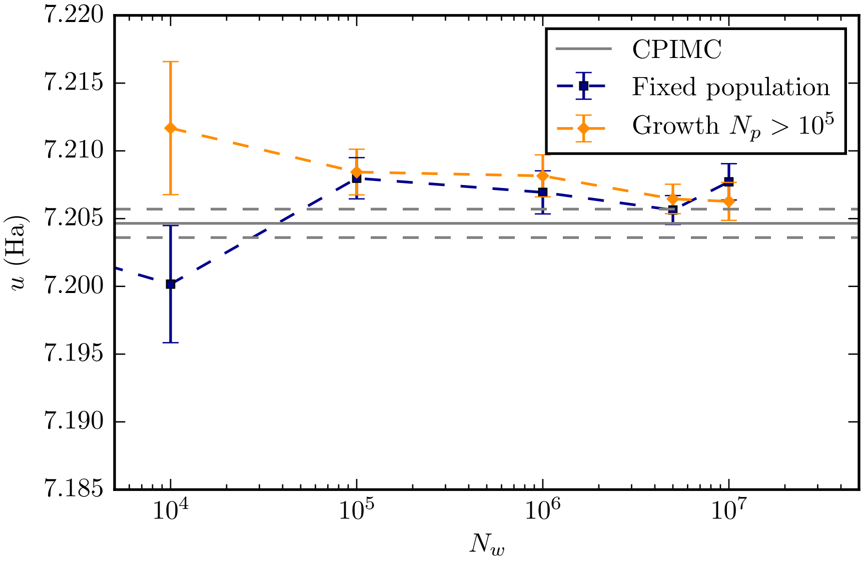


FIG. 3. Convergence of $i$-DMQMC internal energy with target walker population ($N_w$) for $N = 33$, $r_s = 0.6$, $\Theta = 0.5$, $M = 1045$ and $\zeta = 1$. Here we also demonstrate that two methods of population control, i.e., fixing the population at $N_w$ and growing the population to $N_w$ does not have a significant effect on results. Also plotted is the CPIMC result from [8] (solid line) and the corresponding error bar (dashed line).

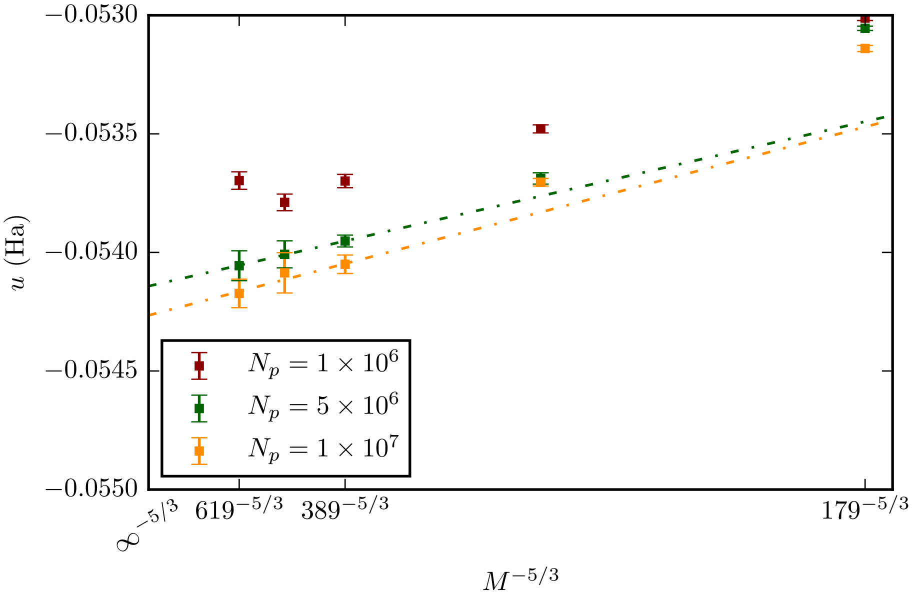


FIG. 4. Convergence of $i$-DMQMC internal energy with target walker population ($N_w$) for $N = 33$, $r_s = 4$, $\Theta = 0.0625$ and $\zeta = 1$. Here, and for the $r_s = 3$ point in Table III, the error is estimated as the difference between the extrapolated values for the two largest populations.

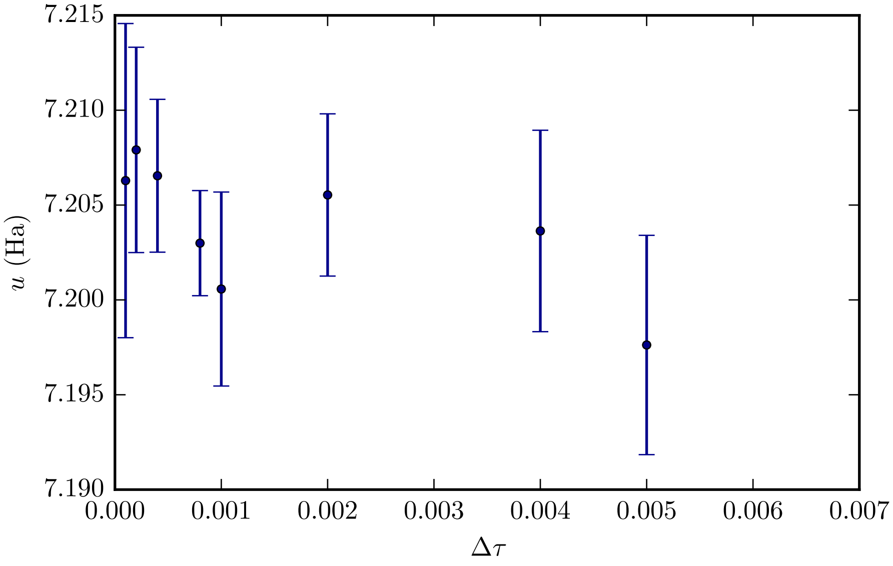


FIG. 5. Variation of internal energy with time step $\Delta\tau$ for $N = 33, \zeta = 1$ and $r_s = 0.6$ at $\Theta = 0.5$ with $M = 751$.

### B. Timestep Bias

At finite temperature using the simple Euler approximation solution for solution to the Bloch equation introduces a time step error which reduces with decreasing temperature [9]. In Fig. 5 we see that any timestep bias is well controlled for the time steps considered in this work.

## II. LOW TEMPERATURE $i$-DMQMC DATA FOR $N = 33$, $\zeta = 1$

In Table II below we list the $i$-DMQMC results for the internal energy ($u$) per-particle for the $N = 33$, $\zeta = 1$ UEG (see main text for definitions). Also listed are the free-electron and various mean field estimates for the internal energy evaluated in the canonical ensemble for the same particle number. In particular, we list $u_0 = \langle \hat{T} \rangle_0 / N$, $u_{\mathrm{HF0}} = \langle \hat{H} \rangle_0 / N$ and $u_{\mathrm{THF}} = \langle \hat{H} \rangle_{\mathrm{THF}} / N$, where $\langle \hat{Y} \rangle_X = Z_X^{-1} \mathrm{Tr}[\hat{Y} \hat{\rho}_X]$ and $Z_X = \mathrm{Tr}[\hat{\rho}_X]$. Here

$$\hat{\rho}_0 = \sum_{\mathbf{i}} e^{-\beta E_{\mathbf{i}}^0} |D_{\mathbf{i}}\rangle\langle D_{\mathbf{i}}|, \tag{1}$$

$$\hat{\rho}_{\mathrm{THF}} = \sum_{\mathbf{i}} e^{-\beta E_{\mathbf{i}}^{\mathrm{HF}}} |D_{\mathbf{i}}\rangle\langle D_{\mathbf{i}}|, \tag{2}$$

where the sum runs over all determinants in a given basis set. For the UEG, $E_{\mathbf{i}}^0 = \langle D_{\mathbf{i}} | \hat{T} | D_{\mathbf{i}} \rangle = \frac{1}{2} \sum_{\mathbf{k}_{\mathrm{occ}}} \mathbf{k}^2$ and $E_{\mathbf{i}}^{\mathrm{HF}} = \langle D_{\mathbf{i}} | \hat{H} | D_{\mathbf{i}} \rangle = E_{\mathbf{i}}^0 - \frac{1}{\Omega} \sum_{\mathbf{k}_{\mathrm{occ}} < \mathbf{p}_{\mathrm{occ}}} \frac{4\pi}{|\mathbf{k} - \mathbf{p}|^2} + \mathrm{const.}$ is the Hartree–Fock energy of determinant $|D_{\mathbf{i}}\rangle$. All mean-field quantities can be evaluated as outlined in [10].

### A. Running Procedure

All simulations used $n_{\mathrm{add}} = 3$. In most simulations we initialised the density matrix with $N_w$ walkers and allowed the shift to vary throughout. For higher densities and the largest walker numbers we instead grew the total population to its target value. Results were averaged over between 20 and a few thousand independent runs depending on the temperature and target population considered. Typical values for the parameters used in our simulations can be found in Table III. We found it efficient to revert to the original asymmetric formulation of DMQMC [10] for $\Theta \leq 0.125$ due to the potentially large weights appearing in the spawning probabilities. However, both approaches produce statistically identical results Fig. 2.

| $r_s$ | $\Theta$ | $u$ | $u_0$ | $u_{\mathrm{HF0}}$ | $u_{\mathrm{THF}}$ |
|---|---|---|---|---|---|
| 0.6 | 0.0625 | 3.8893(2) | 4.9247292(8) | 3.9141788(8) | 3.9098628(8) |
| 0.6 | 0.1250 | 4.1202(8) | 5.169033(3) | 4.169565(3) | 4.136215(2) |
| 0.6 | 0.2500 | 4.9168(9) | 5.990731(7) | 5.038973(8) | 4.931726(7) |
| 0.6 | 0.5000 | 7.208(3) | 8.26458(2) | 7.41292(2) | 7.23096(2) |
| 0.8 | 0.0625 | 1.9895(4) | 2.7701614(5) | 2.0122487(5) | 2.0090903(4) |
| 0.8 | 0.1250 | 2.1167(9) | 2.907581(1) | 2.157980(2) | 2.133328(1) |
| 0.8 | 0.2500 | 2.563(1) | 3.369789(4) | 2.655971(4) | 2.575453(4) |
| 0.8 | 0.5000 | 3.850(3) | 4.64882(1) | 4.01008(1) | 3.87233(1) |
| 1.0 | 0.0625 | 1.1455(2) | 1.7729032(3) | 1.1665729(3) | 1.1641059(3) |
| 1.0 | 0.1250 | 1.225(1) | 1.8608512(9) | 1.261170(1) | 1.2417295(8) |
| 1.0 | 0.2500 | 1.5082(7) | 2.156664(3) | 1.585609(3) | 1.521156(3) |
| 1.0 | 0.5000 | 2.333(1) | 2.975257(7) | 2.464263(7) | 2.353048(8) |
| 1.5 | 0.0625 | 0.36443(9) | 0.7879570(1) | 0.3837369(2) | 0.3821836(1) |
| 1.5 | 0.1250 | 0.3974(6) | 0.8270448(4) | 0.4272576(5) | 0.4147342(4) |
| 1.5 | 0.2500 | 0.523(1) | 0.958517(1) | 0.577814(1) | 0.534846(2) |
| 1.5 | 0.5000 | 0.892(1) | 1.322341(3) | 0.981679(3) | 0.905914(4) |
| 2.0 | 0.0625 | 0.1211(5) | 0.44322576(6) | 0.14006064(9) | 0.13895691(6) |
| 2.0 | 0.1250 | 0.1413(5) | 0.4652125(2) | 0.1653720(3) | 0.1562793(2) |
| 2.0 | 0.2500 | 0.211(2) | 0.5391663(7) | 0.2536388(8) | 0.221480(1) |
| 2.0 | 0.5000 | 0.418(3) | 0.743811(2) | 0.488314(2) | 0.430342(3) |
| 3.0 | 0.0625 | -0.0216(9) | 0.19698921(3) | -0.00512084(3) | -0.00578693(3) |
| 4.0 | 0.0625 | -0.054(1) | 0.11080642(3) | -0.04077613(3) | -0.04123256(3) |

TABLE II. $i$-DMQMC results for the internal energy for the $N = 33, \zeta = 1$ system as well as mean-field Monte Carlo results for the same system in the canonical ensemble. Energies are in Hartree atomic units and contain the Madelung contribution [11].

| $r_s$ | $N_w$ | $M$ | $\Delta\tau \times E_F$ |
|---|---|---|---|
| $< 1$ | $1 \times 10^6$ | 1045 | $1 \times 10^{-3}$ |
| 1 | $5 \times 10^6$ | 1045 | $0.5 \times 10^{-3}$ |
| 2 | $5 \times 10^6$ | 1045 | $0.25 \times 10^{-3}$ |
| $> 2$ | $1 \times 10^7$ | extrap Fig. 4 | $0.25 \times 10^{-3}$ |

TABLE III. Typical parameters used in our $i$-DMQMC simulations. For $r_s \geq 2$, $\Theta \leq 0.125$ we set $n_{\mathrm{ex}} = 0$, i.e., only diagonal elements were permanently set to be initiators.

## III. $i$-FCIQMC

In Fig. 6 below we present the convergence of the $i$-FCIQMC results for the correlation energy per-particle $\varepsilon_c \equiv u(T=0) - u_{\mathrm{HF}}(T=0)$ for $N = 33$ and $r_s = 1$. We see that any remaining initiator error is $\lessapprox 1 \times 10^{-4}$ Ha per-particle and thus negligible for comparison with the finite-temperature results whose error is typically an order of magnitude larger (c.f. Fig. 1 in main text). The Hartree–Fock energy and $i$-FCIQMC correlation energy (extrapolated to the complete basis set limit) for this system are 1.13818594 and $-0.01883(8)$ Ha per-particle respectively. The error in the last digit is due to the extrapolation.

## IV. SYMMETRIC EQUATIONS OF MOTION

In our previous paper [10] we introduced an asymmetric equation of motion for the density matrix, i.e.,

$$\frac{d\hat{f}}{d\tau} = \hat{H}^0 \hat{f} - \hat{f}\hat{H}, \tag{3}$$

for $\hat{f} = e^{-(\beta-\tau)\hat{H}^0} e^{-\tau\hat{H}}$. Eq. (3) leads to an asymmetric algorithm where particles only spawn from one end of the density matrix (i.e., along rows or columns.) While this is formally correct, and the full density matrix should be sampled when $\tau = \beta$, we have found that using the asymmetric algorithm can lead to sampling issues when evaluating observables which do not commute with the Hamiltonian at lower temperatures (Fig. 7). This point was previously

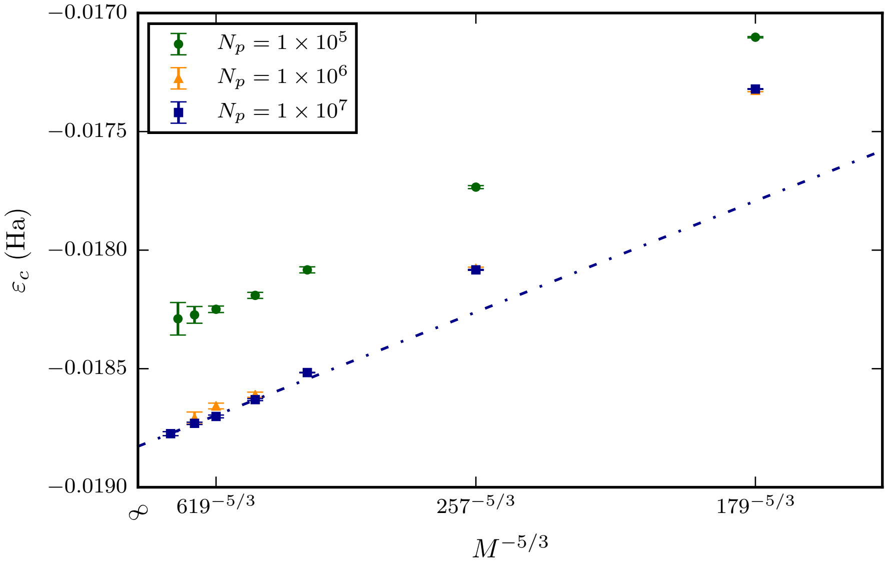


FIG. 6. Convergence of the $i$-FCIQMC correlation energy (per-particle) with basis-set size $M$ and walker number, $N_w$, for $N = 33$, $r_s = 1$ and $\zeta = 1$. Dot-dashed line is a weighted least squares fit [12] of the last four ($N_w = 10^7$) points assuming a $M^{-5/3}$ dependence.

noted in the original DMQMC paper [13], however, explicitly symmetrising Eq. (3) was initially avoided due to the added complications involved.

The symmetric algorithm listed in the main text follows by setting

$$\hat{f} = e^{-\alpha \hat{H}^0} e^{-\tau \hat{H}} e^{-\alpha \hat{H}^0}, \tag{4}$$

$$\frac{d\hat{f}}{d\tau} = \frac{1}{2}\{\hat{H}^0, \hat{f}\} - \frac{1}{2}(\hat{H}_I(-\alpha)\hat{f} + \hat{f}\hat{H}_I(\alpha)), \tag{5}$$

for $\alpha = \frac{1}{2}(\beta - \tau)$. In Fig. 7 we see it performs much better at lower temperatures. The computational cost for the symmetric algorithm is typically greater than its asymmetric counterpart due to the added exponentiation required as well as increasing the stochastic noise at low temperatures due to potentially large walker population fluctuations. Optimizing this algorithm and investigating improved initiator approximations is a current area of research.

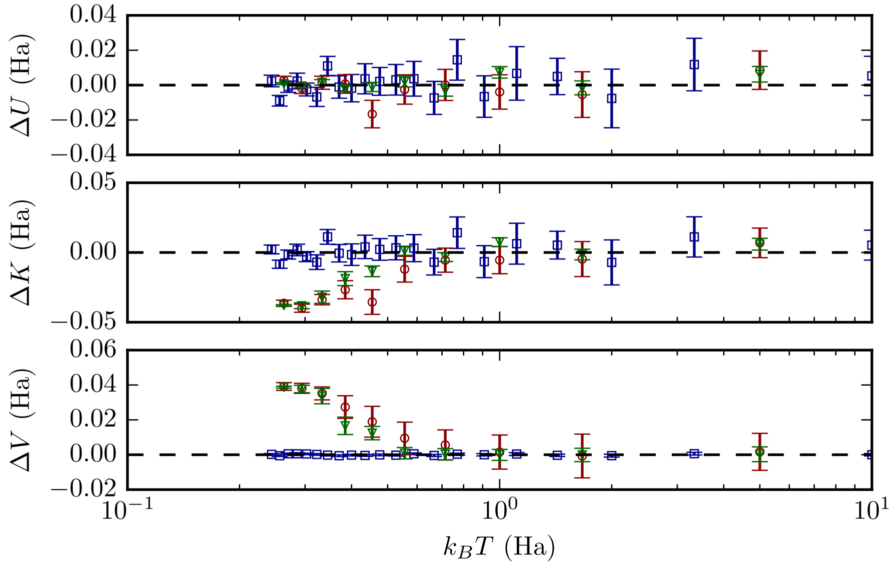


FIG. 7. Deviation of internal, kinetic (here denoted $K$ to avoid confusion with the temperature $T$) and potential energy from exact (FCI) values for symmetric (blue squares) and asymmetric (red circles and green triangles) equations of motion. We see that the symmetric equations perform much better at lower temperatures which is largely a sampling issue. This can be seen when increasing the target walker population by a factor of 10 (green triangles). Note that both methods produce exact results for observables which commute with the Hamiltonian. The system shown here is $N = 7$, $M = 19$ and $\zeta = 1$.

## V. FREE ENERGIES

The Helmholtz free energy

$$F = U - TS \tag{6}$$
$$= -k_BT \log Z \tag{7}$$

can be estimated in DMQMC as follows. Define

$$\tilde{F}(\tau) = -k_BT \log Z(\tau) \tag{8}$$
$$= -k_BT \log \mathrm{Tr}[\hat{f}(\tau)], \tag{9}$$

for $\hat{f}$ defined as in Eq. (4) with $\tilde{F}(\tau = 0) = F_0$ and $\tilde{F}(\tau = \beta) = F$. Differentiating Eq. (9) with respect to $\tau$ we find

$$\frac{d\tilde{F}}{d\tau} = -k_BTZ(\tau)^{-1}\mathrm{Tr}\Big[\frac{d\hat{f}}{d\tau}\Big], \tag{10}$$
$$= -k_BTZ(\tau)^{-1}\mathrm{Tr}[(H^0 - H(-\alpha))\hat{f}], \tag{11}$$
$$= k_BT\langle\hat{V}_I(-\alpha)\rangle_\tau, \tag{12}$$

where we have inserted Eq. (5) for $\frac{d\hat{f}}{d\tau}$ and used the cyclicity of the trace and the definition of $\hat{V}_I(-\alpha) = e^{-\alpha\hat{H}^0}\hat{V}e^{\alpha\hat{H}^0} = e^{-\alpha\hat{H}^0}(\hat{H} - \hat{H}^0)e^{\alpha\hat{H}^0} = \hat{H}_I(-\alpha) - \hat{H}^0$ in arriving at Eq. (12). Finally, integrating Eq. (12) we find

$$F_{\mathrm{xc}} = k_BT\int_0^\beta \langle V_I(-\alpha)\rangle_\tau \; d\tau, \tag{13}$$

as claimed in the main text.

### A. Basis set corrections

To alleviate the slow convergence of $f_{\mathrm{xc}}$ with basis size at higher temperatures we use mean-field basis set corrections similar to those developed in [10]. Here we add a first order correction to $f_{\mathrm{xc}}$, $\Delta f_{\mathrm{x}}^0 = v_0(\infty) - v_0(M)$ where $v_0 =$

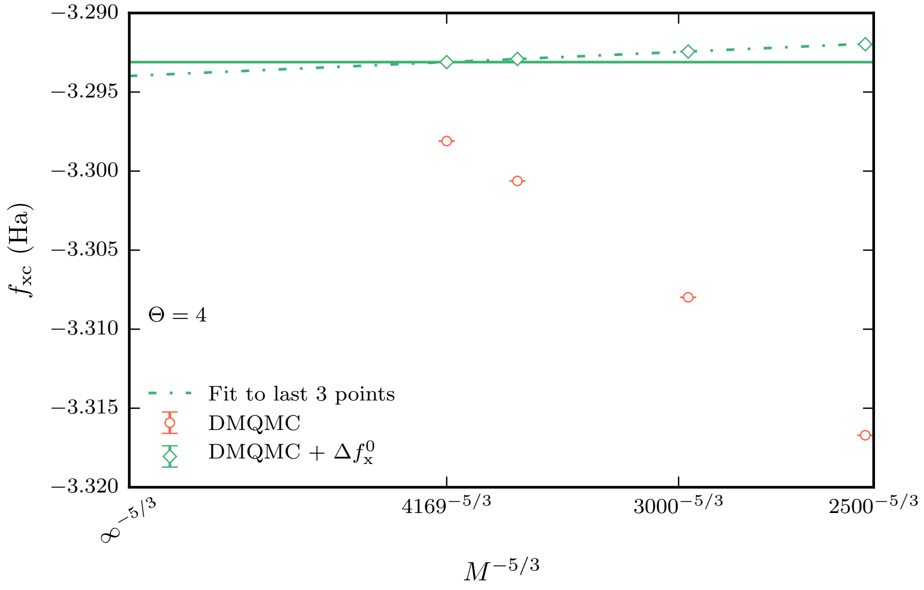


FIG. 8. Basis set corrections applied to DMQMC data for $f_{\rm xc}$ for $N = 33, \zeta = 1, r_s = 0.1, \Theta = 4$ showing the reduction in overall basis set error when corrections are applied. Here we can reach an estimated accuracy of $\approx 2$ mHa per electron estimated as the difference between the maximum DMQMC data point considered at $M = 4169$ plane waves (horizontal line) and the extrapolated value (dot-dashed line). The extrapolation was performed using a weighted least squares fit [12] assuming a $M^{5/3}$ behaviour to the last 3 points.

$N^{-1}\langle \hat{V} \rangle_0$ is the first order exchange contribution to the free energy. A demonstration of the effectiveness of this procedure for $f_{\rm xc}$ is shown in Fig. 8 and the corrections which were applied are listed in Table IV.

| $r_s$ | $\Theta$ | $M$ | $\Delta u_{\rm HF}$ | $\Delta f_{\rm x}^0$ |
|---|---|---|---|---|
| 0.1 | 1 | 4169 | 0.000(2) | 0.000001(3) |
| 0.1 | 2 | 4169 | 0.107(4) | 0.000021(3) |
| 0.1 | 4 | 4169 | 39.70(1) | 0.004996(2) |
| 0.1 | 8 | 4169 | 707.01(3) | 0.043527(1) |
| 0.6 | 1 | 1935 | 0.00018(5) | 0.0000010(6) |
| 0.6 | 2 | 1935 | 0.2114(1) | 0.0004830(4) |
| 0.6 | 4 | 4169 | 1.1003(3) | 0.0008330(3) |
| 0.6 | 8 | 4169 | 19.6350(9) | 0.0072550(2) |
| 1.0 | 1 | 1935 | 0.00008(2) | 0.0000010(3) |
| 1.0 | 2 | 1935 | 0.07557(4) | 0.0002910(3) |
| 1.0 | 4 | 4169 | 0.3954(1) | 0.0005000(2) |
| 1.0 | 8 | 4169 | 7.0675(3) | 0.0043530(1) |
| 2.0 | 4 | 4169 | 0.09838(3) | 0.00025000(9) |
| 2.0 | 8 | 4169 | 1.76566(8) | 0.00217600(6) |

TABLE IV. Basis set corrections applied to DMQMC data listed in Hartrees. $M$ is the basis set size used in the corresponding DMQMC calculation.

### B. High temperature free energy data

| $r_s$ | $\Theta$ | $u$ | $u_0$ | $u_{\rm xc}$ | $f$ | $f_0$ | $f_{\rm xc}$ |
|---|---|---|---|---|---|---|---|
| 0.1 | 1 | 489.20(1) | 494.663(1) | -5.46(1) | -318.7188(2) | -314.3278(2) | -4.39100(4) |
| | 2 | 912.40(2) | 916.898(3) | -4.50(2) | -1288.8046(5) | -1285.0719(4) | -3.73267(3) |
| | 4 | 1778.47(3) | 1782.254(9) | -3.79(4) | -3823.638(1) | -3820.340(1) | -3.29310(1) |
| | 8 | 3524.63(5) | 3527.98(3) | -3.35(6) | -10099.676(2) | -10096.597(4) | -3.035181(6) |
| 0.6 | 1 | 12.789(1) | 13.74057(3) | -0.951(1) | -9.498698(6) | -8.731327(5) | -0.76737(6) |
| | 2 | 24.671(1) | 25.46940(7) | -0.798(1) | -36.34776(1) | -35.69644(1) | -0.65084(1) |
| | 4 | 48.845(1) | 49.5070(3) | -0.662(1) | -106.68992(3) | -106.12058(3) | -0.568508(9) |
| | 8 | 97.425(1) | 98.0006(9) | -0.575(2) | -280.98500(6) | -280.4609(1) | -0.516817(4) |
| 1.0 | 1 | 4.369(4) | 4.94662(1) | -0.578(4) | -3.617375(3) | -3.143278(2) | -0.4741(8) |
| | 2 | 8.671(1) | 9.16907(3) | -0.498(1) | -13.253807(4) | -12.850722(4) | -0.40279(3) |
| | 4 | 17.409(1) | 17.82261(9) | -0.414(1) | -38.55380(1) | -38.20341(1) | -0.34988(2) |
| | 8 | 34.9274(5) | 35.2806(3) | -0.3532(6) | -101.28553(2) | -100.96604(4) | -0.315136(3) |
| 2.0 | 4 | 4.235(1) | 4.45565(2) | -0.220(1) | -9.735757(2) | -9.550846(3) | -0.1847(1) |
| | 8 | 8.6325(4) | 8.81992(8) | -0.1874(4) | -25.407175(5) | -25.24150(1) | -0.16350(1) |

TABLE V. DMQMC results for the internal and free energy for the $N = 33, \zeta = 1$ system as well as ideal results for the same system in the canonical ensemble. Energies are in Hartree atomic units and contain the Madelung contribution where appropriate [11]. Errors listed are purely stochastic in nature; we estimate that the basis set error for $\Theta \geq 4$ is at most 3 mHa per electron for $f_{\rm xc}$.

[1] D. Cleland, G. H. Booth, and A. Alavi, J. Chem. Phys. **132**, 041103 (2010).
[2] G. H. Booth, D. Cleland, A. J. Thom, and A. Alavi, J. Chem. Phys. **135**, 084104 (2011).
[3] D. Cleland, G. H. Booth, C. Overy, and A. Alavi, J. Chem. Theory Comput. **8**, 4138 (2012).
[4] R. E. Thomas, G. H. Booth, and A. Alavi, Phys. Rev. Lett. **114**, 033001 (2015).
[5] J. J. Shepherd, G. H. Booth, and A. Alavi, J. Chem. Phys. **136**, 244101 (2012).
[6] J. J. Shepherd, G. Booth, A. Grüneis, and A. Alavi, Phys. Rev. B **85**, 081103 (2012).
[7] G. H. Booth, A. Grüneis, G. Kresse, and A. Alavi, Nature **493**, 365 (2013).
[8] T. Schoof, S. Groth, J. Vorberger, and M. Bonitz, Phys. Rev. Lett. **115**, 130402 (2015).
[9] G. H. Booth, A. J. W. Thom, and A. Alavi, J. Chem. Phys. **131**, 054106 (2009).
[10] F. D. Malone, N. S. Blunt, J. J. Shepherd, D. K. K. Lee, J. S. Spencer, and W. M. C. Foulkes, J. Chem. Phys. **143**, 044116 (2015).
[11] L. M. Fraser, W. M. C. Foulkes, G. Rajagopal, R. J. Needs, S. D. Kenny, and A. J. Williamson, Phys. Rev. B **53**, 1814 (1996).
[12] E. Jones, T. Oliphant, P. Peterson, *et al.*, (2001–), [Online; accessed 2016-02-10].
[13] N. S. Blunt, T. W. Rogers, J. S. Spencer, and W. M. C. Foulkes, Phys. Rev. B **89**, 245124 (2014).
